# Supplementary material for: Report on the Third Workshop on Sustainable Software for Science: Practice and Experiences (WSSSPE3)
Source: arXiv:1602.02296 source file (2016-02-06)
Supplement: Supplementary file 2 [file wg_appendix_legacy_SW.tex]

%%%%%%%%%%%%%%%%%%%%%%%%%%%%%%%%%%%%%%%%%%%%%%%%%%%%%%%%%%%%
\section{Legacy Software Working Group Discussion}
\label{sec:appendix_legacy_SW}
%%%%%%%%%%%%%%%%%%%%%%%%%%%%%%%%%%%%%%%%%%%%%%%%%%%%%%%%%%%%

\todo{add POC here}

\subsection{Group Members}

\begin{itemize}
\item name -- affiliation
\item name2 -- affiliation2
\end{itemize}

\subsection{Summary of Discussion}

\subsection{Description of Opportunity, Challenges, and Obstacles}

\subsection{Key Next Steps}

\subsection{Plan for Future Organization}

\subsection{What Else is Needed?}

\subsection{Key Milestones and Responsible Parties}

\subsection{Description of Funding Needed}
